# Supplementary material for: Imprinted atomic displacements drive spin-orbital order in a vanadate perovskite
Source: arXiv:2409.12871 source file (2024-09-19)
Supplement: Supplementary file 1 [file Radhakrishnan_SupplMater.pdf]

# Supplemental Material for ”Imprinted atomic displacements drive spin-orbital order in a vanadate perovskite”

P. Radhakrishnan,[1] K. S. Rabinovich,[1] A. V. Boris,[1] K. Fürsich,[1] M. Minola,[1] G. Christiani,[1] G. Logvenov,[1] B. Keimer,[1] and E. Benckiser[1,*]

[1] *Max Planck Institute for Solid State Research, Heisenbergstrasse 1, 70569 Stuttgart, Germany*

This document provides additional details and measurements that support the main manuscript.

## I. CHARACTERIZATION AND STRUCTURAL ANALYSIS

The $YVO_3$ (YVO) thin films, grown on $YAlO_3$ (YAO), $NdGaO_3$ (NGO) and $DyScO_3$ (DSO) orthorhombic substrates were investigated by x-ray diffraction (XRD) using a Cu-$K_{\alpha_1}$ lab source. The results are summarised in Fig. S1 (a-d).

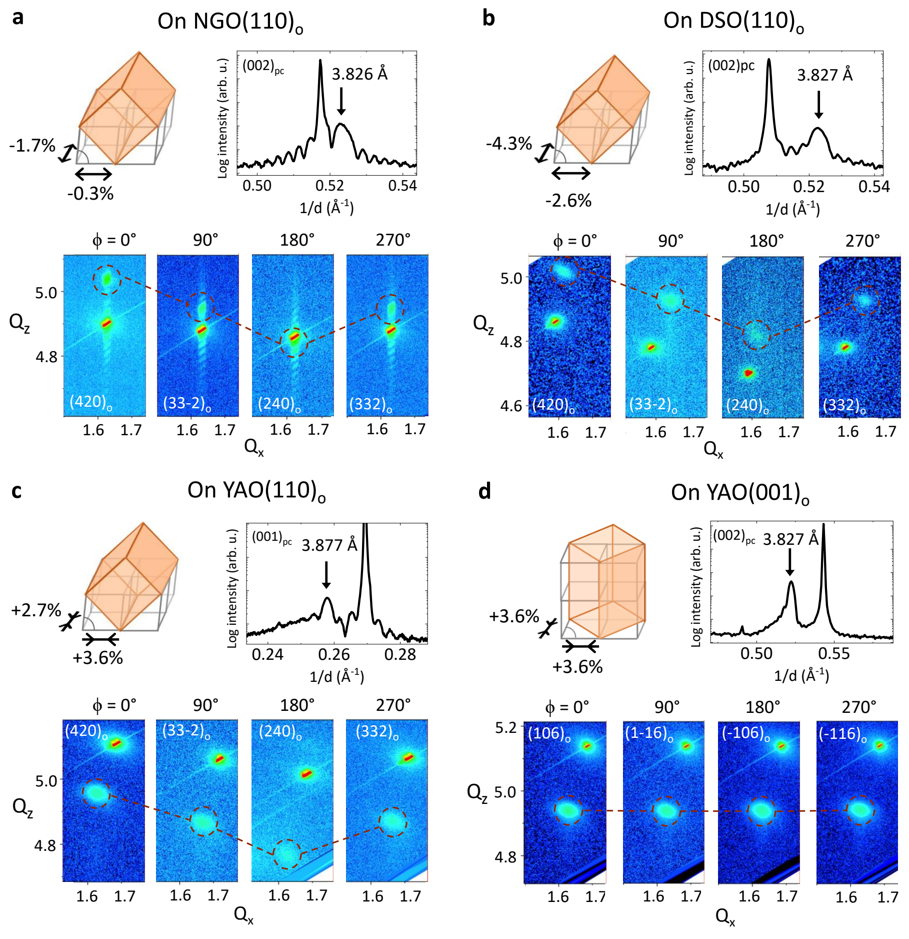


FIG. S1. Characterization by x-ray diffraction of YVO thin films on (a) NGO$(110)_o$ (b) DSO$(110)_o$ (c) YAO$(110)_o$ and (d) YAO$(001)_o$ substrates. The schematic on the top left displays the orientation of the orthorhombic unit cell (orange), where the smaller (grey) cubes correspond to the pseudocubic unit cells. The lattice mismatch [1] of YVO with each substrate is stated in the schematic. For each part (a-d), the top right and bottom panels show the out-of-plane XRD scans and RSMs of the pseudocubic {103} family of in-plane reflections measured at azimuthal angle ($\phi$) 90 degrees apart, respectively. The Miller indices indicated for each map refer to the orthorhombic space group (*Pbnm*). The dashed circles mark the positions of the film peaks.

* E.Benckiser@fkf.mpg.de

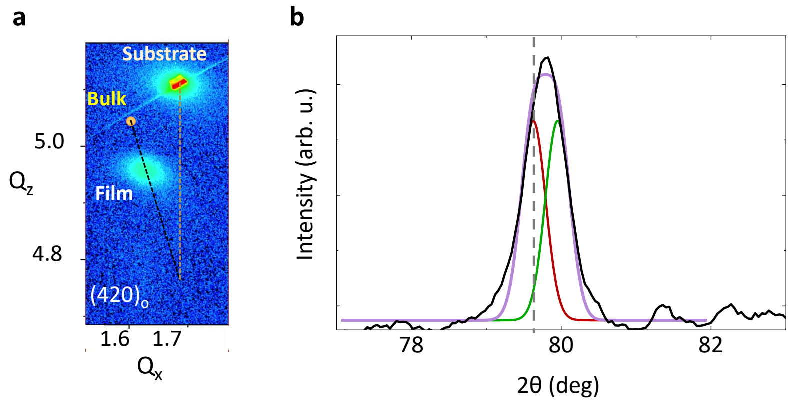


FIG. S2. (a) Reciprocal space map of *Pbnm*-(420) reflection of YVO film on YAO$(110)_o$. The relaxation line (dashed black) is the line that passes through the bulk YVO peak position (orange) and the center of the film peak. (b) Scan of the film peak along the relaxation line. We fit this peak with two Gaussians, the grey dashed line marks the position of the Gaussian peak corresponding to the strained portion of the film.

While YVO is under tensile strain on NGO$(110)_o$ and DSO$(110)_o$, it experiences compressive strain on YAO$(110)_o$ and YAO$(001)_o$. Hence for YVO films on NGO$(110)_o$ and DSO$(110)_o$, the out-of-plane parameters are smaller compared to the corresponding bulk pseudocubic value of 3.85 Å, whereas it is larger for the film on YAO$(110)_o$. Likewise, for compressive strain on YAO$(001)_o$, the out-of-plane parameter is larger than the bulk pseduocubic value of 3.79 Å (indicated in the top right panels of Fig. S1, next to the arrows).

We used reciprocal space maps (RSM) to examine the epitaxial orientation of the orthorhomobic YVO unit cell and the strain state of thin films. Comparing all the samples, we observe that only the film on NGO$(110)_o$ is fully strained, since it has the same $Q_x$ value as the substrate [Fig. S1(a)]. The films on DSO$(110)_o$, YAO$(110)_o$, and YAO$(001)_o$ are partially relaxed due to the much larger lattice mismatch on these substrates [Fig. S1(b-d)]. We determined the unit cell orientation of the films using the azimuthal dependence of the pseudocubic {103} family of reflections. For films grown on $(110)_o$-oriented substrates [Fig. S1(a-c)], the film and substrate peak positions display a characteristic pattern through the change in the azimuthal angle, which indicate that the orthorhombic $c$-axis of both are parallel and in the plane of the sample surface ($\phi$) [2]. In contrast, for the sample on YAO$(001)_o$ [Fig. S1(d)], the substrate

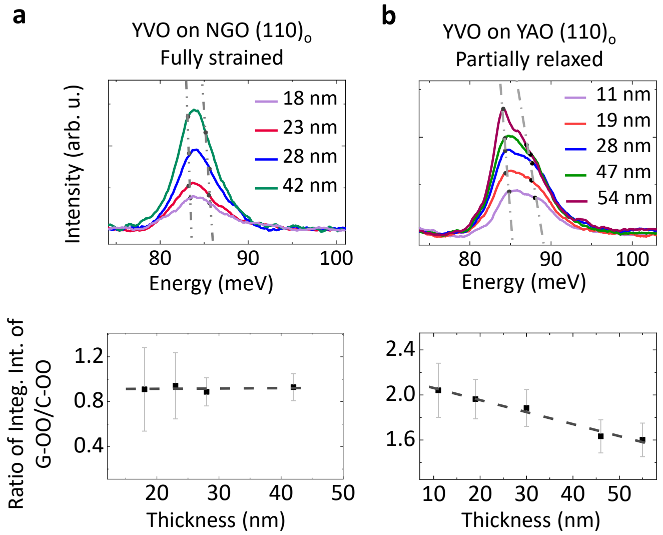


FIG. S3. Spectra of the $B_{1g}$ mode at 20 K for YVO films with different thicknesses (a) on NGO$(110)_o$ and (b) on YAO$(110)_o$. All data were collected at a setpoint temperature of 20 K, however since a weaker filter was used in the case of the film on NGO, it has some laser heating effects (see text). (c,d) Ratio of integrated areas of the $G$-OO phonon and the $C$-OO phonon with linear fit for the YVO film on NGO$(110)_o$ and YAO $(110)_o$, respectively. The error bars for the ratios were estimated by the propagation of error of the integrated intensities of $C$-OO and $G$-OO phonons.

and film peaks fall in a nearly straight line, through the change in $\phi$, indicating that here the orthorhombic $c$-axis of YVO is out-of-plane with respect to the sample surface. Thus, the orientation of the YVO-$Pbnm$ unit cell follows that of the substrate facet in all cases.

Fig. S2 displays the reciprocal space map of the $(420)_o$ reflection (left) and the scan performed along the relaxation line of the YVO film on YAO$(110)_o$ (right). To be consistent with the Raman measurements, where we focused on the contribution of the strained part of the films (see main text), we fit the relaxation line scan with two Gaussians, corresponding to contributions from strained and relaxed portions of the film. For the fitting process, the FWHM (full width at half maximum) of the two Gaussians were kept equal and fixed at roughly half the value of the entire peak. Their areas were also kept equal and then the Gaussian peak positions were fitted to obtain the lattice parameter of the strained part of the film. From this procedure, we obtained orthorhomobic lattice parameters $b$ = 5.61 Å, $c$ = 7.53 Å for YVO on YAO$(110)_o$ and $b$ = 5.57 Å, $c$ = 7.66 Å for YVO on YAO$(001)_o$, respectively.

## II. THICKNESS DEPENDENCE

We examined the thickness dependence of two sets of films under different degrees of strain. Fig. S3(a,b) shows the $B_{1g}$ phonons at 20 K for YVO films of different thicknesses on NGO$(110)_o$ and YAO$(110)_o$, respectively. The dashed grey lines (top panel) are a linear fit of the centers of the $C$-OO and $G$-OO phonons.

The films on YAO$(110)_o$ [Fig. S3(b), top] show a clear increase in the energy of the phonon peaks with decreasing thickness. In comparison, for the films on NGO [Fig. S3(a), top], the phonons do not show such a pronounced energy dependence with the change in thickness. A shift in the phonon peak positions with thickness indicates a variable amount of strain in the films [3], which is consistent with the fact that the films on NGO$(110)_o$ and the films on YAO$(110)_o$ are fully strained and partially relaxed, respectively.

The bottom panels of Fig. S3 display the ratio of the integrated intensities of the $G$-OO mode to $C$-OO mode as a function of thickness. In the case of the films on NGO$(110)_o$, we observed that the ratio is more or less constant with thickness. In contrast, for the films on YAO$(110)_o$, we saw a decreasing trend of the ratio with thickness, with thinner films having a larger amount of $G$-OO phase relative to $C$-OO phase. This implies that the relaxed portion of the film has bulk-like behaviour and contributes to the $C$-OO peak intensity. Thus, partial relaxation must at least partly create the observed phase coexistence at low temperatures in the films on YAO$(110)_o$. Note that due to time constraints, the films on NGO$(110)_o$ were measured using a weaker filter, corresponding to a higher laser power

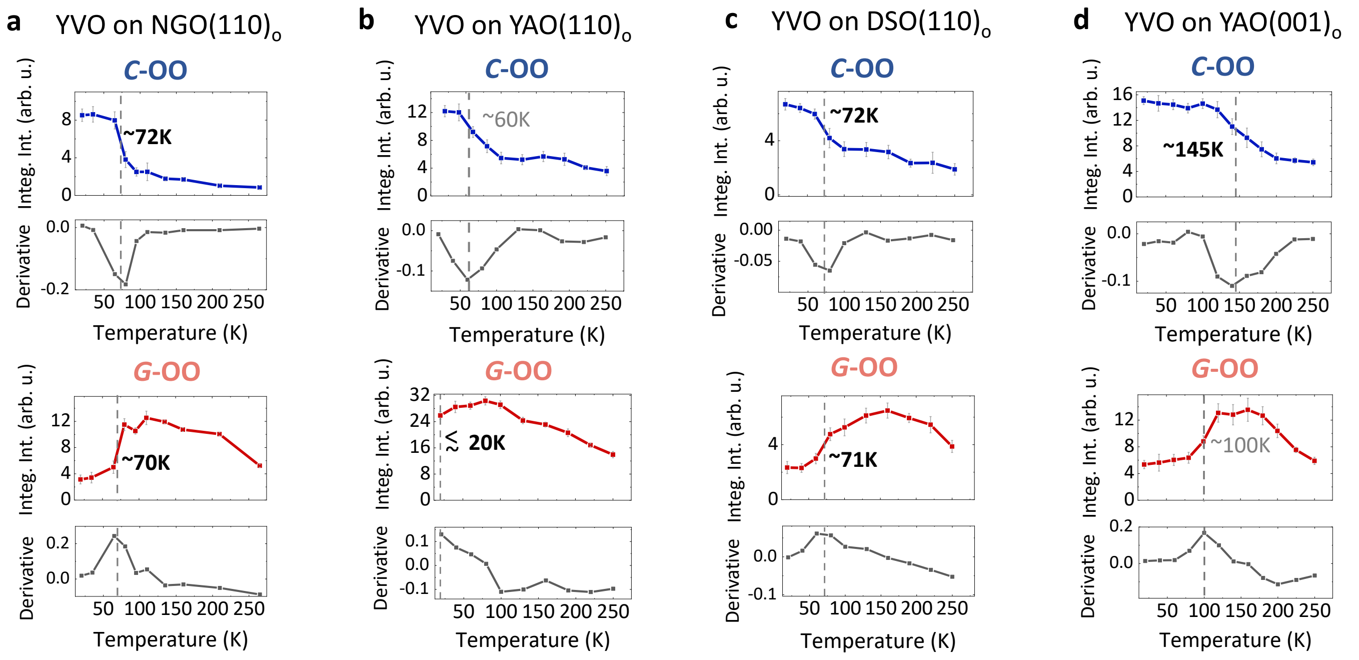


FIG. S4. Temperature dependence and their derivatives for the $C$-OO and $G$-OO modes of YVO films on (a) NGO$(110)_o$, (b) YAO$(110)_o$, (c) DSO$(110)_o$, and (d) YAO$(001)_o$ substrates. The grey and black $T_{\mathrm{OO2/SO2}}$ values in (b, d) correspond to the portion of the film under smaller and larger degrees of strain, respectively.

of $\sim 2.5\,\text{mW}$. Therefore, the true temperature of the sample is expected to be higher than 20 K, but since we are only examining the thickness dependence of the phonon peak positions and intensities, the shift in temperature is not consequential.

## III. DETERMINATION OF TRANSITION TEMPERATURES FROM RAMAN SPECTRA

Since there is an abrupt change in intensity of the $C$-OO and $G$-OO modes across the $G$-SO/$C$-OO to $G$-OO/$C$-SO first-order phase transition, we identified this temperature using the derivative of the integrated intensities of the two modes. The minimum/maximum of the derivative is relatively sharp and thus requires a large data point density for an accurate determination of the temperature. Therefore, we roughly estimated the temperature of transition by considering the center of the full width at half maximum of the derivative (Fig. S4). The drop (rise) in intensity of the $C$-OO ($G$-OO) mode is less sharp for the partially relaxed films on YAO$(110)_o$, YAO$(001)_o$ and DSO$(110)_o$, compared to the fully strained film on NGO$(110)_o$. This is explained by the strain gradient present in these films, due to which, different parts within the sample may undergo transitions at different temperatures, leading to the observed broadening. As explained in the main text, for the films on YAO$(110)_o$ and YAO$(001)_{oo}$ which exhibit a stabilization of the $G$-OO and $C$-OO phases, respectively, a mismatch exists between the $T_{\text{OO2/SO2}}$ values derived from the $C$-OO and $G$-OO modes. The strain-induced phase stabilization effect gradually decreases going from the film-substrate interface towards the top of the film, as the degree of partial relaxation increases. This understanding is supported by the fact that for the partially relaxed film on DSO$(110)_o$, that does not stabilize either phase, there is almost no mismatch between the $T_{\text{OO2/SO2}}$ values obtained from the $C$-OO and $G$-OO modes.

## IV. TEMPERATURE DEPENDENCE OF OPTICAL SPECTRA

We analyze the temperature dependence of the optical spectra by integrating the difference in optical conductivity, defined as $\Delta\sigma_1^c = \sigma_1^c(T) - \sigma_1^c(10\text{ K})$. By studying the difference of $\sigma_1^c$, we focus solely on the temperature dependent changes in the optical spectra [4] and eliminate the contribution of the high energy bands (above $\sim 4.5$ eV), which are largely temperature independent.

Fig. S5(a) displays the $\Delta\sigma_1^c$ spectra at 100 K for YVO films on DSO$(110)_o$ (39 nm) and YAO$(110)_o$ (48 nm). At 3.2 eV, $\Delta\sigma_1^c$ changes sign, which marks the energy range (0 - 3.2 eV) of peak A and B (high-spin multiplet). Due

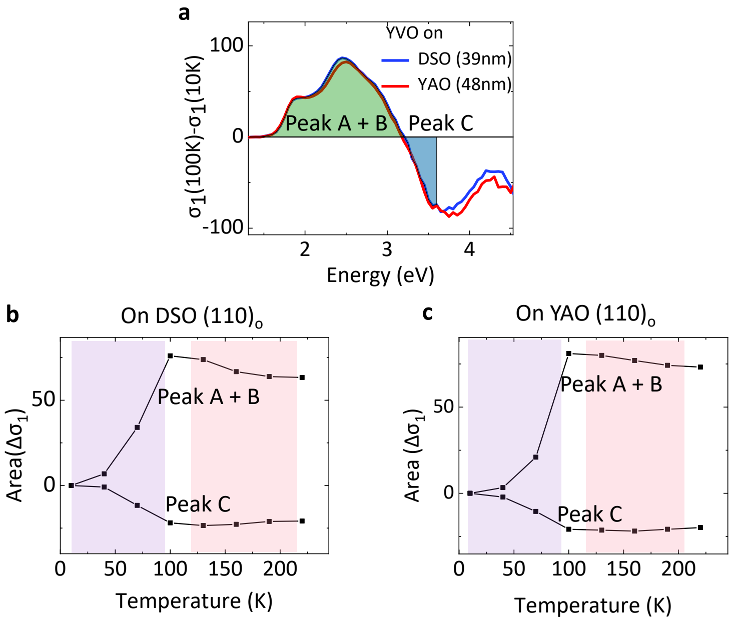


FIG. S5. Temperature dependence of optical conductivity $\sigma_1^c$ measured along the $c$-axis of YVO films on DSO$(110)_o$ (39 nm thickness) and YAO$(110)_o$ (48 nm thickness). (a) $\sigma_1^c(100\,K) - \sigma_1^c(10\,K)$ for both films, displaying energy regions of peaks A and B (high-spin) from 0 to 3.2 eV and peak C (low-spin) from 3.2 to 3.6 eV. (b, c) Temperature dependence of integral of $\sigma_1^c(T) - \sigma_1^c(10\,K)$ of peaks A + B and peak C for films on DSO$(110)_o$ and YAO$(110)_o$, respectively.

to the proximity of peak C (low-spin multiplet) to peak D ($t_{2g}$ to $e_g$ transition), it is not possible to separate their independent contributions, therefore we use the energy value assigned in bulk YVO (3.2 - 3.6 eV) for peak C [5]. Fig. S5(b, c) displays the temperature dependence of the $\Delta\sigma_1^c$ integral for the films on YAO$(110)_o$ and DSO$(110)_o$, respectively. The trends of peaks A+B and peak C are similar to bulk YVO [5], i.e. peaks A+B and peak C have the opposite temperature dependence, since they correspond to high-spin and low-spin multiplets, respectively. The region highlighted in purple shows the first order transition at $T_{\mathrm{OO2/SO2}}$. The part highlighted in pink, displays a decrease in the integrated intensity of peak A+B. This corresponds to the reduction in spin and orbital correlations as we approach the transitions at $T_{\mathrm{SO1}}$ from $C$-SO to paramagnetic state and at $T_{\mathrm{OO1}}$, from $G$-OO to disordered state. Since both of these are second-order phase transitions, they only appear as small kinks in the spectra of bulk YVO, and thus the exact transition temperatures could not be discerned with the temperature intervals measured for the films.

[1] Frank, F. C., Van Der Merwe, J. H. & Mott, N. F. One-dimensional dislocations. ii. misfitting monolayers and oriented overgrowth. *Proc. R. Soc. A* **198**, 216–225 (1949).

[2] Vailionis, A. *et al.* Misfit strain accommodation in epitaxial $AB$O$_3$ perovskites: Lattice rotations and lattice modulations. *Phys. Rev. B* **83**, 064101 (2011).

[3] Hepting, M., Kukuruznyak, D., Benckiser, E., Le Tacon, M. & Keimer, B. Raman light scattering on ultra-thin films of LaNiO$_3$ under compressive strain. *Phys. Rev. B Condens. Matter* **460**, 196–198 (2015).

[4] Kovaleva, N. N. *et al.* Spin-controlled Mott-Hubbard bands in LaMnO$_3$ probed by optical ellipsometry. *Phys. Rev. Lett.* **93**, 147204 (2004).

[5] Reul, J., Nugroho, A. A., Palstra, T. T. M. & Grüninger, M. Probing orbital fluctuations in $R$VO$_3$ = Y, Gd, or Ce) by ellipsometry. *Phys. Rev. B* **86**, 125128 (2012).
